# Supplementary material for: Acc-SpMM: Accelerating General-purpose Sparse Matrix-Matrix Multiplication with GPU Tensor Cores
Source: arXiv:2501.09251 source file (2025-01-16)
Supplement: Supplementary file 1 [file Appendix.tex]

\section{Related Work}

We provide Acc-SpMM's source code.

\subsection{Artifact Summary}

Dataset: Provided in source code folder dataset.
Runtime environment: Ubuntu 20.04 or higher.
Hardware: Multicore x86\_64 CPU with one or more NVIDIA GPUs.
Metrics: Speedups.

\subsection{Description}
